# Supplementary material for: MPC with Learned Residual Dynamics with Application on Omnidirectional MAVs
Source: arXiv:2207.01451 source file (2022-07-04)
Supplement: Supplementary file 1 [file 08_appendix.tex]

% \section{Appendix}
% More plots that could be used.
% \begin{figure}[ht]
%     \includegraphics[width=\columnwidth]{plots/21_Power.pdf}\caption{Power comparison for optimal and non-optimal allocation.}\label{fig:powerComparison}
% \end{figure}

% \begin{figure}[ht]
%     \includegraphics{plots/21_23_Tiltangle_rate_comparison.pdf}\caption{Comparison of tilt angle speeds for constrained AMPC and unconstrained WMPC. AMPC mean: $0.577\pm\SI{0.326}{\radian\per\second}$, WMPC mean: $0.808\pm \SI{0.857}{\radian\per\second}$}\label{fig:tiltAngleRateComparison}
% \end{figure}

% \begin{figure}[ht]
%     \includegraphics[width=\columnwidth]{plots/deviation_violinplot.pdf}\caption{Deviations of variables from optimal values.}\label{fig:AMPCdeviations}
% \end{figure}
